# Supplementary material for: Giant field enhancement by funneling effect into sub-wavelength slit-box resonators
Source: arXiv:1403.2198 source file (2014-03-10)
Supplement: Supplementary file 1 [file article_prl_helm_suppsv2.pdf]

# Giant field enhancement by funneling effect into sub-wavelength slit-box resonators

Paul Chevalier,[1,2] Patrick Bouchon,[2,*] Riad Haïdar,[2,3] and Fabrice Pardo[1,†]

[1]*Laboratoire de Photonique et de Nanostructures (LPN-CNRS), Route de Nozay, 91460 Marcoussis, France*

[2]*ONERA, The French Aerospace Lab, 91761 Palaiseau, France*

[3]*École Polytechnique, Département de Physique, 91128 Palaiseau, France*

(Dated: March 9, 2014)

## Abstract

Supplementary materials concerning the high field intensity enhancement in the slit-box resonators. The method used for the simulations is described in this paper, and specific formulas are derived.

## SUPPLEMENTARY MATERIALS

### Materials and Methods

*Simulations*

All the simulations have been performed with a vectorial method [1]. The dielectric function of gold is computed from the Drude model $\varepsilon_{\rm Au}(\lambda) = 1 - [(\lambda_p/\lambda + i\gamma)\,\lambda_p/\lambda]^{-1}$ which matches well the experimental data for $\lambda_p = 159\,\text{nm}$ and $\gamma = 0.0077$ [2].

The computations have been verified with COMSOL-Multiphysics to check and confirm the convergence of the method.

*Focusing*

In order to simulate a beam focused onto a single structure, we decompose a focused gaussian beam into 75 propagative plane waves. The simulated situation is obtained by linearly recomposing the simulations obtained for the different plane waves.

### Comparison between the slit-box resonator and a Fabry Perot model

In the Fig. S 1(a) we respectively present the reflectivity spectra of a grating of open slits and a slit-box resonator having the same resonance wavelength and repeated with the same period. This spectra is plotted until the lower bound of the validity of the Drude model of gold. This figure shows the presence of harmonic resonance with the open slit structure that do not appear for the slit box structure.

The electric field distribution inside the slit is also non uniform and significantly decreases at the center of the structure as shown in Fig. S 1(b-c). This property does not appear for the slit-box structure where the electric field remains constant along the height of the slit.

The reasons for theses difference is that the two resonances have two different mechanisms. In the case of the open slit it is described by a Fabry Perot, by considering the effective index of the waveguide and its reflection coefficient. However for the slit-box resonator only the LC model describes and explains the resonance presented in the article and the large field intensity enhancement associated with the resonance. The cavity has inductive properties

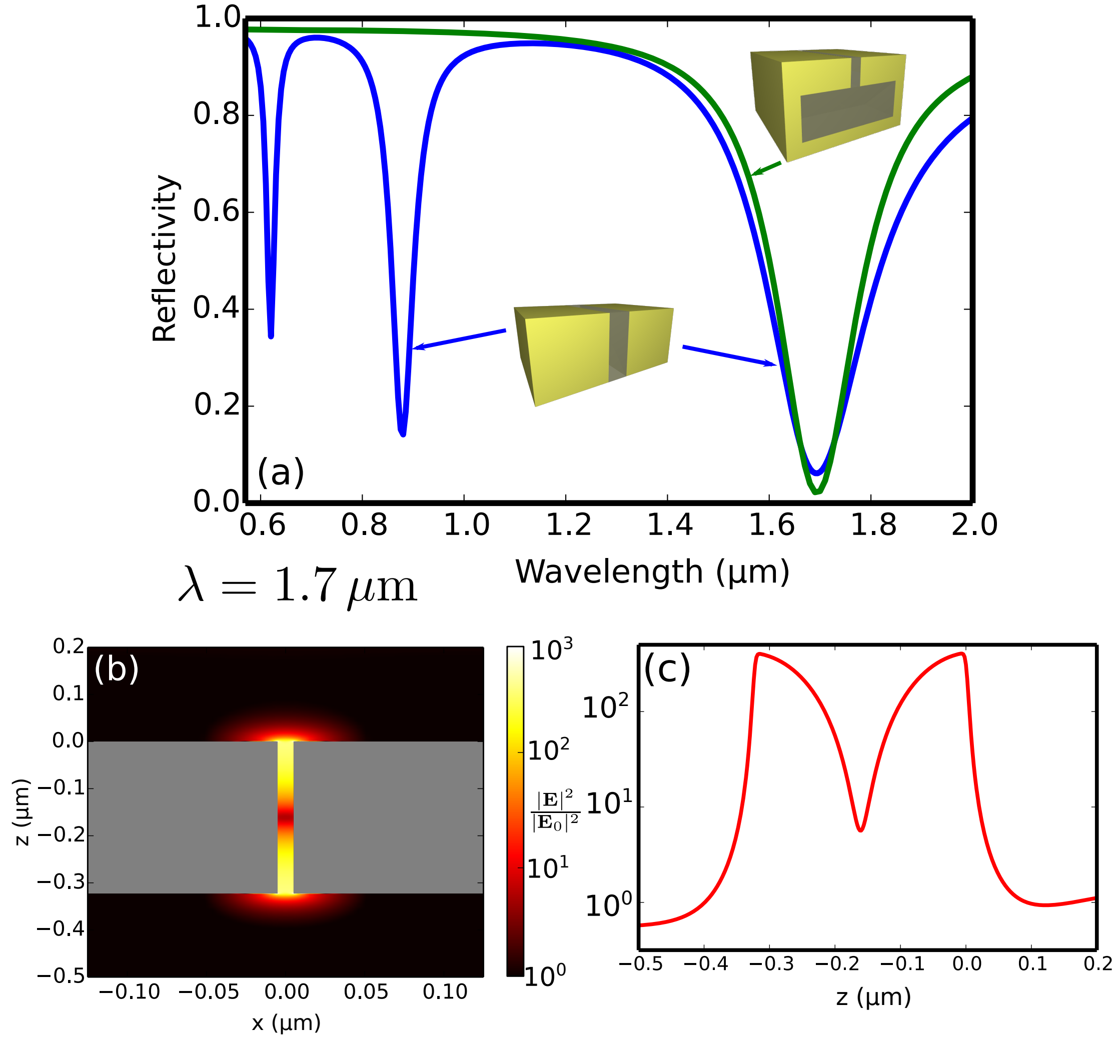


Figure S 1. (a) Reflectivity spectra of an open slit structure of width $w = 10$ nm and of height $h = 322$ nm (blue line), compared to the reflectivity spectra of the slit-box structure studied in the article and presented in Fig.2 (green line) ; both with a period $d = 250$nm. The two structures have the same resonance wavelength ($1.7\,\mu$m), but only the open slits presents harmonic resonances. (b) Field intensity enhancement for the open slit structure at the resonance (c) The field at the center of the open slit is plotted as a function of $z$.

and stores magnetic energy which explains why the slit-box resonator cannot be restricted to it electric field.

**Magnetic field**

For the structure presented in the article the actual field map of the magnetic field intensity is shown in figure S 2. Compared to the electric field (see figure 2.C-D), the magnetic field is far less enhanced (at least 3 orders of magnitude less in the slit. This indicate that the funneling effect contribute very little to the enhancement of the magnetic field. In the cavity, the enhancement is uniform which can be explained by the fact that it behaves as the inductance (and therefore stores half the energy) which underlines the role played by the box as a magnetic energy accumulator. The non-uniform enhancement in the slit can thus be explained as a side effect of the continuity of the magnetic field.

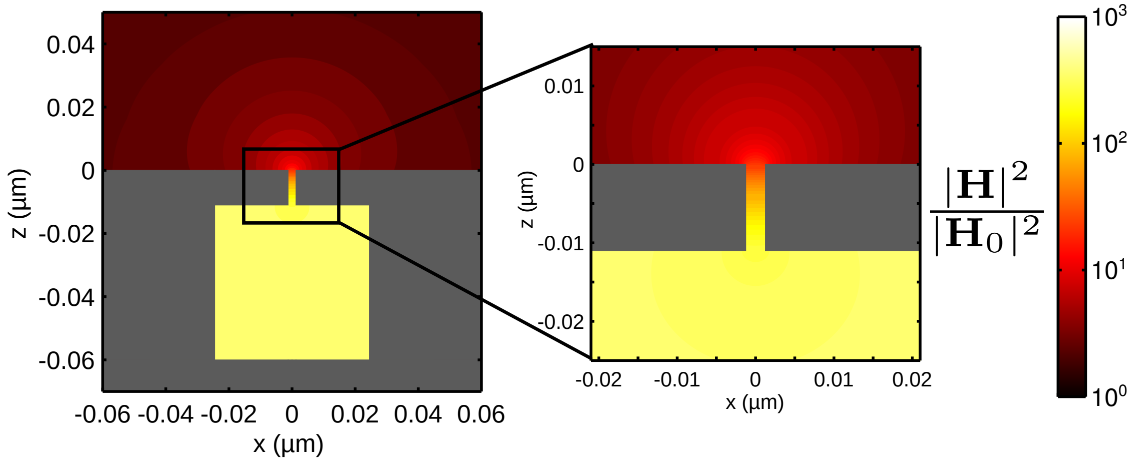


Figure S 2. Magnetic field intensity map for the structure presented in the article : $w_b = 49\,\text{nm}$, $h_b = 49\,\text{nm}$, $h_s = 11\,\text{nm}$, $w_s = 2.5\,\text{nm}$, plotted for a wavelength $\lambda = 1.7\,\mu\text{m}$.

**Enhancement at other wavelengths**

The total funneling of light into subwavelength slit-box resonators actually provides giant field intensity enhancement, and this concept could be extended to other wavelengths, as shown in the following examples. In order to increase the enhancement, the width of the slit should be reduced, but to maintain the same level of absorption in the structure and the same resonance wavelength the height of the slit should be reduced. Two limits exists for the size of the slits: if its height is too small, the concept of slit barely exists and the cavity is no more isolated from the outside so we choose slit at least 12 nm tall (half of the skin

depth). In order to neglect quantum effect, slits of width greater than 2 nm are also chosen. The two following examples show stronger field intensity enhancement within those limits, at different wavelength that we compare to existing realizations in the literature. Designing such resonators at visible wavelengths is actually possible but could require the material used for the side walls to have a smaller plasma wavelength (e.g. using silver instead of gold).

*At* 15 $\mu$m

As presented in figure S 3, we optimize a structure that totally absorbs light at a wavelength of 15 $\mu$m with a slit of width $w_s = 2\,\text{nm} = \lambda/7500$. On the field map we see that the total electric field intensity is enhanced by a factor $10^6$. The structure is such that $w_b = 485\,\text{nm}$, $h_b = 485\,\text{nm}$, $h_s = 30\,\text{nm}$. The quality factor of the resonance is about 10, and the period is $d = 3\,\mu\text{m}$.

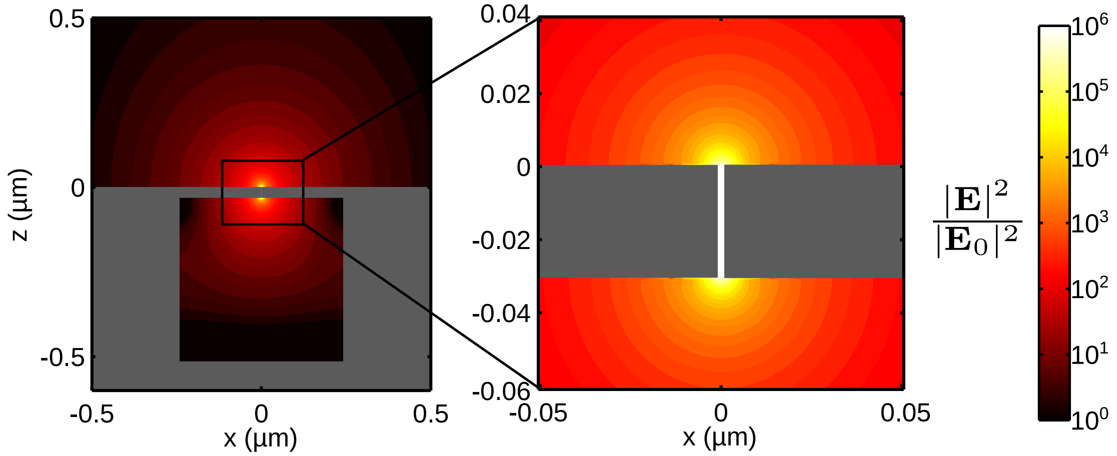


Figure S 3. Electric field intensity map inside a structure where : $w_b = 485\,\text{nm}$, $h_b = 485\,\text{nm}$, $h_s = 30\,\text{nm}$, $w_s = 2\,\text{nm}$. A field intensity enhancement of $10^6$ is reached inside the slit at a wavelength of 15 $\mu$m.

*At* 200 $\mu$m

In the THz domain, we can even reach higher field intensity enhancement due to lower losses in the metal in this regime. As presented in figure S 4, we design a structure with a

resonance at 200 $\mu$m with a slit of width $w_s = 4\,\text{nm} = \lambda/50000$ that presents a field intensity enhancement of $10^8$. The structure is such that $w_b = 5.65\,\mu\text{m}$, $h_b = 5.7\,\mu\text{m}$, $h_s = 80\,\text{nm}$. The quality factor of the resonance is about 20, and the period is $d = 50\,\mu\text{m}$. The field intensity enhancement is here stronger than presented in the literature at similar wavelengths [3, 4].

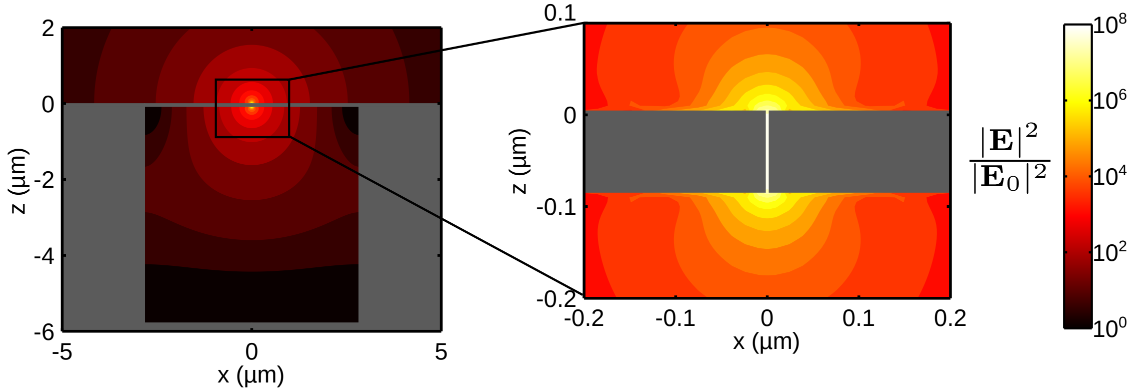


Figure S 4. Electric field intensity map inside a structure where : $w_b = 5.65\,\mu\text{m}$, $h_b = 5.7\,\mu\text{m}$, $h_s = 80\,\text{nm}$, $w_s = 4\,\text{nm}$. A field intensity enhancement of $10^8$ is reached inside the slit at a wavelength of 200 $\mu$m.

**Analytical model for the resonance wavelength**

A rough approximation of the resonance wavelength can be derived depending on the geometric parameters of the structure. The narrow slit actually behaves like a capacitor where the electric field is homogeneous, the capacity of the equivalent capacitor for a fixed section of length $T$ in the $\mathbf{y}$ direction is therefore :

$$C = \varepsilon_0 \varepsilon_s \frac{h_s T}{w_s} \tag{1}$$

The cavity however behaves like an inductance of surface $S_b = w_b h_b$ :

$$L = \mu_0 \frac{w_b h_b}{T} \tag{2}$$

The resonance wavelength is therefore :

$$\lambda_R = 2\pi c \sqrt{LC} = 2\pi n_s \sqrt{\frac{h_s}{w_s} h_b w_b} \tag{3}$$

By using a refined formula for the capacity where the height of the slit is replaced by an effective height $h_s + w_s$ to take into account the edge effect near the capacitor, the resonance wavelength writes :

$$\lambda_R = 2\pi c\sqrt{LC} = 2\pi n_s \sqrt{\frac{h_s + w_s}{w_s} h_b w_b} \tag{4}$$

Simulations made in the near and middle IR domain for $n_s = 1$ are presented in figure S 5. They show that the formula gives actually a rather good approximation. The simulations are made for 2000 different structures where $w_s$ is between 10 nm and 60 nm, $h_s$ is between 50 nm and 200 nm, $w_b$ is between 100 nm and 600 nm, $h_b$ is between 100 nm and 600 nm, and $d$ is 2 $\mu$m and 4 $\mu$m.

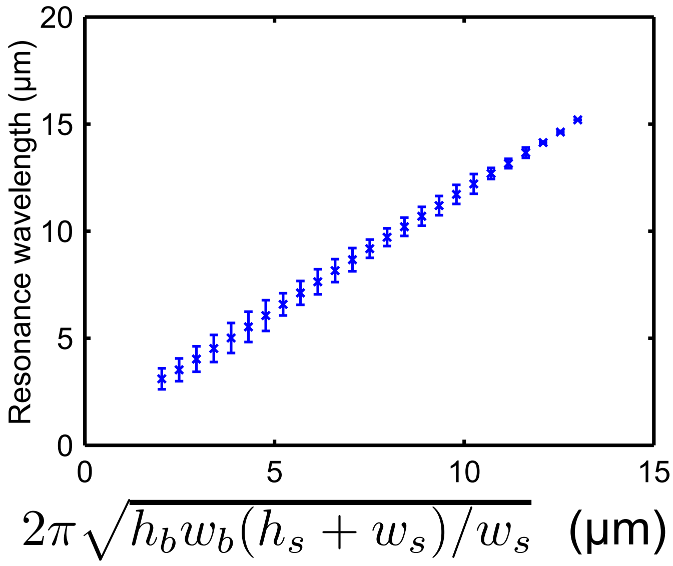


Figure S 5. Simulations for different size of structure (and $n_s = 1$) have been realized. For each structure the resonance wavelength is computed by simulation and is compared to the model provided here. We see a strong correlation between the simulations results and the predicted resonance wavelength for the structure we simulated.

**Acoustics and Electromagnetism**

As shown in Fig. S6A, the Helmholtz resonator is composed by a large cavity with a small aperture. The resonator is three-dimensional (3D) with a tubular bottleneck. This tube,

having a diameter much smaller than the wavelength, is able to propagate an acoustic wave. This is not the case for an electromagnetic wave, which has a vectorial nature. Therefore the Helmholtz resonators (acoustic 3D geometries) cannot be applied to electromagnetism. However, bidimensional electromagnetic problems are scalar and the analogy between optics and acoustics can apply [5]. The resonators studied in the manuscript long enough along the **y** direction to be considered as infinite and consists of a box (surface $S_b$) and a slit (width $w_s$, height $h_s$) as shown in Fig. S6B. In acoustics, such 2D Helmholtz resonator can be modelized (as in 3D) by a mass-spring resonator: the mass of the air contained in the neck oscillates and compresses the air in the cavity. A resonance wavelength is easily derived from this model [6–8]:

$$\lambda_R = 2\pi\sqrt{\frac{S_b h_s}{w_s}}, \tag{5}$$

and is similar to the one obtained above. It shows that $\lambda_R$ depends on the characteristic dimension of the box $\sqrt{S_b}$ and on the slit aspect ratio $\sqrt{h_s/w_s}$. The electromagnetic structure which is considered in the following is made of a metallic material with a similar geometry, the slit is filled by a dielectric material of relative permittivity $\varepsilon_s$, and the box is filled with a magnetic material of relative permeability $\mu_b$. In a quasi-static approximation, this structure can be viewed as a LC resonator as shown in Fig. S6C: the coil is made of one loop, having an area $S_b$, filled with the magnetic material and the capacitor has plates of height $h_s$, spaced by $w_s$ filled with the dielectric material which justifies the previous derivation.

The acoustic and electrical systems give similar formulas, one based on the mass-spring model and the other based on the LC model. The two systems have in common the wave equation with boundary conditions on the walls of the slit and the box.

Indeed, for a two dimensional electromagnetic problem invariant by translation under the $y$ direction, the magnetic field is along the $y$ axis and the electric field is in the $zx$ plane. The problem is described by the set of equations:

$$\Delta \mathbf{E} + \varepsilon\mu \frac{\partial^2 \mathbf{E}}{\partial t^2} = 0 \tag{6}$$

and

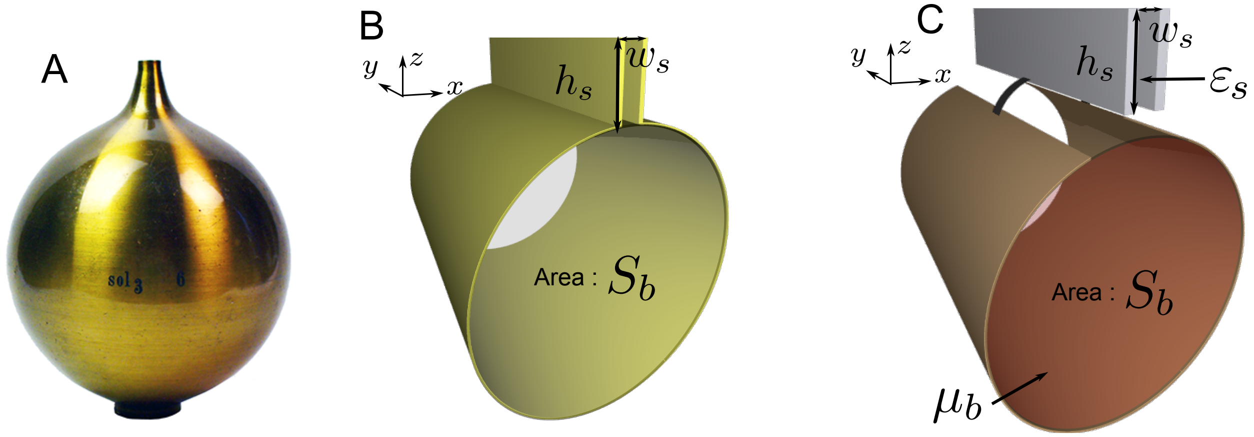


Figure S 6. (A) Acoustic Helmholtz resonator. (B) Two-dimensional Helmholtz resonator infinite in the $\mathbf{y}$ direction, with a slit of height $h_s$ and width $w_s$, and a box of area $S_b$. (C) LC resonator made with a two dimensional capacitor and coil. Both components are infinite and behave ideally at all frequencies.

$$\mathrm{div}(\mathbf{E} \wedge \mathbf{y}) = \mathrm{rot}\mathbf{E} \cdot y = -\mu \frac{\partial H_y}{\partial t} \tag{7}$$

For a linearized acoustic problem, the set of equation verified by the acoustics speed $\mathbf{u}$ and pressure field $p$ (for linearized problems) writes:

$$\Delta \mathbf{u} + \chi \rho_0 \frac{\partial^2 \mathbf{u}}{\partial t^2} = 0 \tag{8}$$

$$\mathrm{div}(\mathbf{u}) = -\chi \frac{\partial p}{\partial t} \tag{9}$$

And both perpendicular electric field $(\mathbf{E} \wedge \mathbf{y})$ and acoustic speed verifies similar boundary conditions. This shows the analogy between acoustics and electromagnetic variables as specified in the following table.

| | | Acoustics | Electromagnetism |
|---|---|---|---|
| Fields | | Acoustic speed | $\mathbf{E} \wedge \mathbf{y}$ |
| | | Acoustic pressure | $\mathbf{H}_y$ |
| Constitutive parameters | Slit | Fluid density | $\varepsilon$ |
| | Box | Compressibility | $\mu$ |

The density of the air in the slit plays a similar role as the relative dielectric permittivity, while the compressibility of the air can be assimilated to the relative magnetic permeability. It must be emphasized that the analogy still stands for boundary conditions: the acoustic speed is zero and so is $\mathbf{E} \wedge \mathbf{y}$ for a perfect metal. Optical resonators that could be modeled by simple LC circuits under the quasistatic approximation have already been shown in optics under the name of split ring resonators [9], those resonators are used to design metamaterials [10] or to engineer spectral filtering [11]. The structure presented in the following is different from split ring resonators since it is coupled to the free space only through the aperture of the resonators.

**Field intensity enhancement**

By considering the absorption coefficient $A$ of the structure, the quality factor of the resonance links the incident energy and the stored energy.

$$\frac{Q}{2\pi} = \frac{E_{\text{stored}}}{E_{\text{dissipated per period}}} \tag{10}$$

The maximum electric field intensity is linked to the maximum difference of potential $V$ in the capacitor such that $|V| \simeq |E| w_s$, so the stored energy in the resonator is :

$$E_{\text{stored}} = \frac{1}{2} C |E|^2 w_s^2 = \frac{1}{2} \varepsilon_0 \varepsilon_s \frac{h_s T}{w_s} |E|^2 w_s^2 \tag{11}$$

For a slice of the resonator of thickness $T$, the energy dissipated per temporal period, is equal to the incident power divided by the frequency $\nu$ and normalized by the absorption coefficient :

$$E_{\text{dissipated per period}} = \frac{A|S_0|dT}{\nu} = \frac{A}{2\nu}|E_0||H_0|dT = \frac{\lambda}{2Z_0 c} A|E_0|^2 dT = \frac{\lambda \varepsilon_0}{2} A|E_0|^2 dT \tag{12}$$

Therefore :

$$\frac{Q}{2\pi} = \frac{\varepsilon_0 \varepsilon_s \frac{h_s T}{w_s} |E|^2 w_s^2}{\lambda \varepsilon_0 A |E_0|^2 dT} = \frac{\varepsilon_s h_s w_s |E|^2}{\lambda d A |E_0|^2} \tag{13}$$

So the field intensity enhancement could be expressed by :

$$\frac{|E|^2}{|E_0|^2} = \frac{QA\lambda d}{2\pi\varepsilon_s h_s w_s} \tag{14}$$

Given that the energy absorption efficiency could be at most of 1 in optimized situations, and for a normally incident plane wave we can achieve this optimum for $d \leq \lambda$ so that the maximum field intensity enhancement is:

$$\frac{|E|^2}{|E_0|^2} = \frac{Q\lambda^2}{2\pi\varepsilon_s h_s w_s} \tag{15}$$

This is the formula written is the manuscript that does not give the exact value for a specific structure but rather an asymptotic boundary that could be approached.

---

* patrick.bouchon@onera.fr

† fabrice.pardo@lpn.cnrs.fr

[1] P. Bouchon, F. Pardo, R. Haïdar, and J. Pelouard, Journal of the Optical Society of America A **27**, 696 (2010).

[2] E. Palik and G. Ghosh, *Handbook of optical constants of solids* (Academic press, 1985).

[3] C. Feuillet-Palma, Y. Todorov, A. Vasanelli, and C. Sirtori, Scientific Reports **3** (2013).

[4] M. Seo, H. Park, S. Koo, D. Park, J. Kang, O. Suwal, S. Choi, P. Planken, G. Park, N. Park, *et al.*, Nature Photonics **3**, 152 (2009).

[5] A. Sommerfeld, *Optics Lectures on Theortical Physics, vol. IV*, Vol. 1 (Academic Press INC, New York, NY, 1954).

[6] L. Rayleigh, *The theory of sound*, Vol. 2 (Macmillan, 1896).

[7] L. Rayleigh, Proceedings of the Royal Society of London. Series A **92**, 265 (1916).

[8] H. von Helmholtz, *Theorie der Luftschwingungen in Röhren mit offenen Enden*, 80 (W. Engelmann, 1896).

[9] T. Meyrath, T. Zentgraf, and H. Giessen, Physical Review B **75**, 205102 (2007).

[10] J. Pendry, A. Holden, D. Robbins, and W. Stewart, Microwave Theory and Techniques, IEEE Transactions on **47**, 2075 (1999).

[11] R. Marques, J. Martel, F. Mesa, and F. Medina, Physical Review Letters **89**, 183901 (2002).
